# Supplementary material for: RIGI: Rectifying Image-to-3D Generation Inconsistency via Uncertainty-aware Learning
Source: arXiv:2411.18866 source file (2024-11-28)
Supplement: Supplementary file 1 [file 6_suppl.tex]

\clearpage
\setcounter{section}{0}
\maketitlesupplementary

\begin{figure*}[!t]
\centerline{\includegraphics[width=0.85\textwidth]{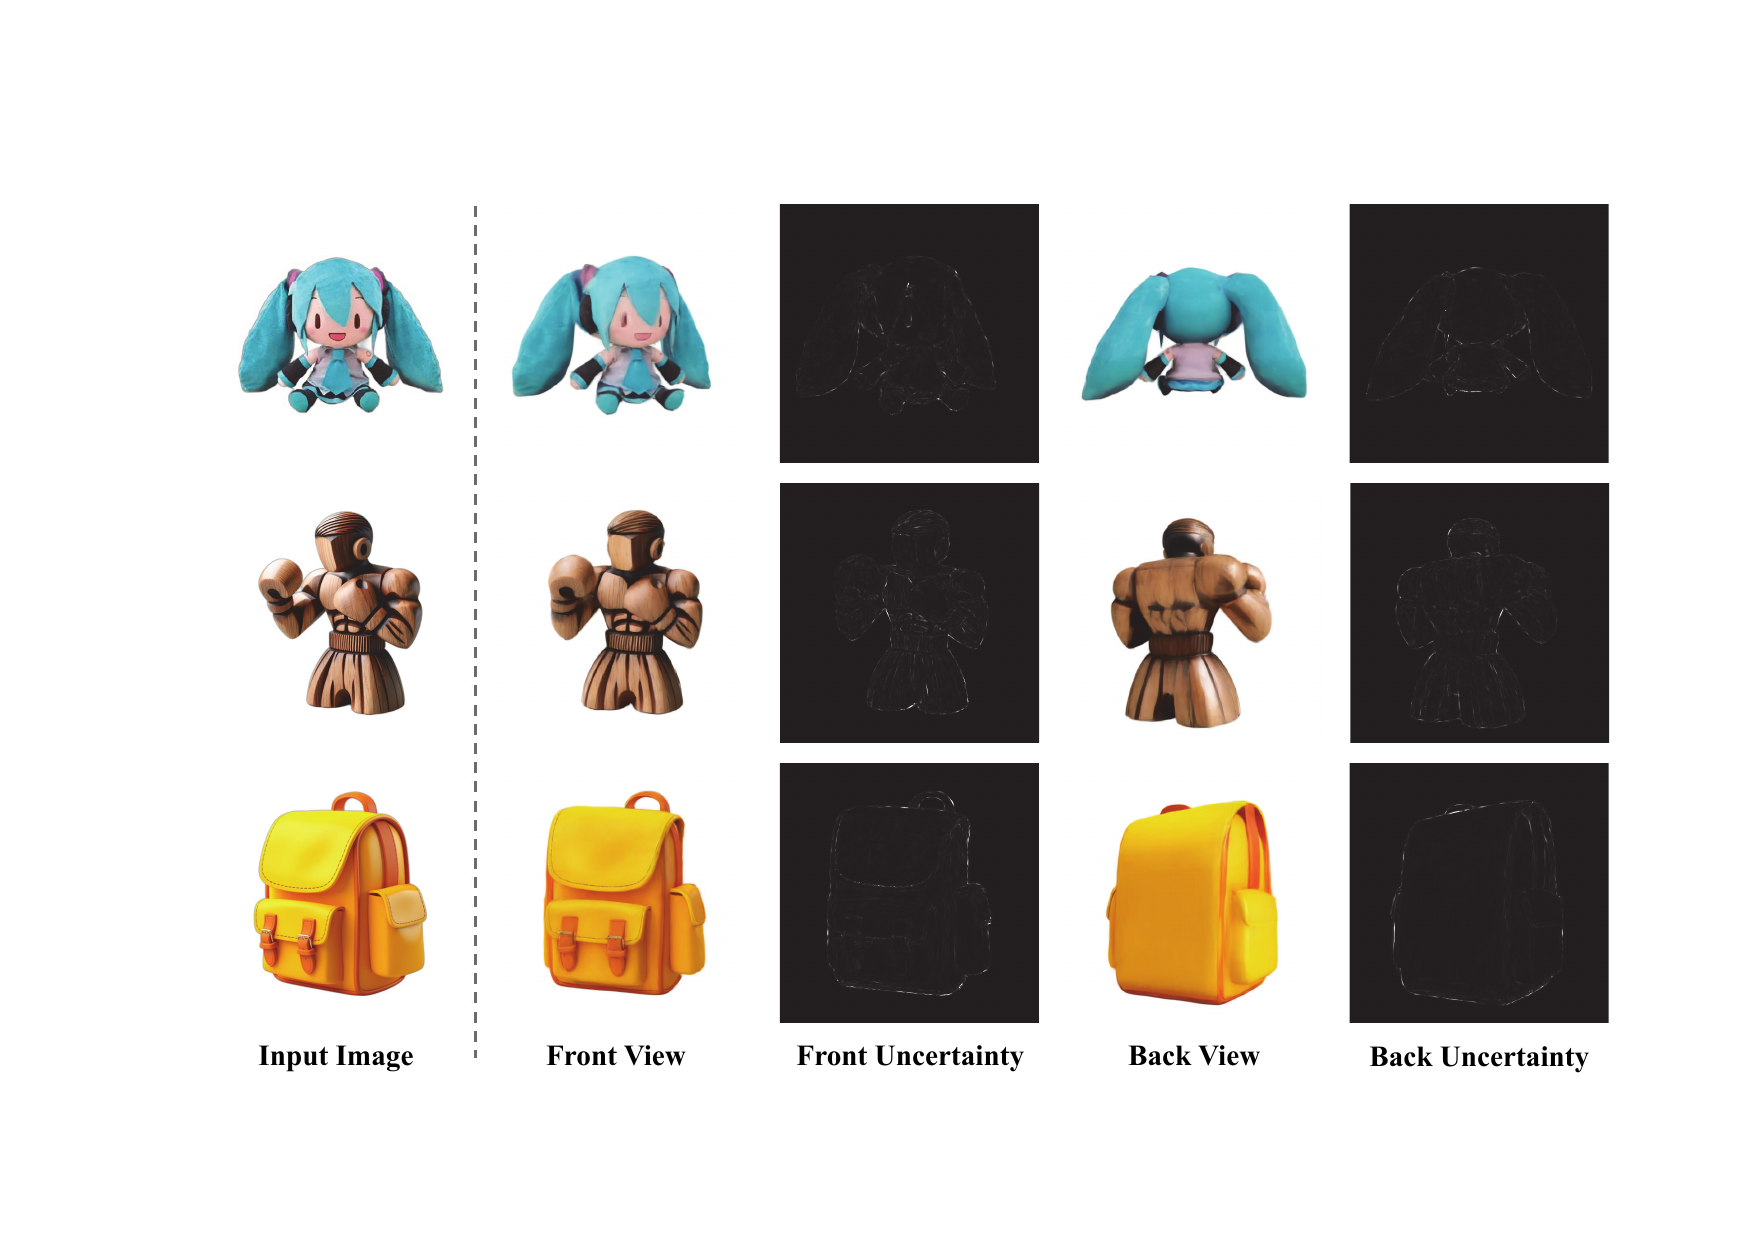}}
\caption{Visualization of the Uncertainty Map. The estimated uncertainty map highlights higher values in edge and sharp-texture regions, effectively capturing the inconsistencies present in the pseudo labels.}
\label{fig:suppl_vis_uncert}
\end{figure*}

\begin{figure*}[!t]
\centerline{\includegraphics[width=0.85\textwidth]{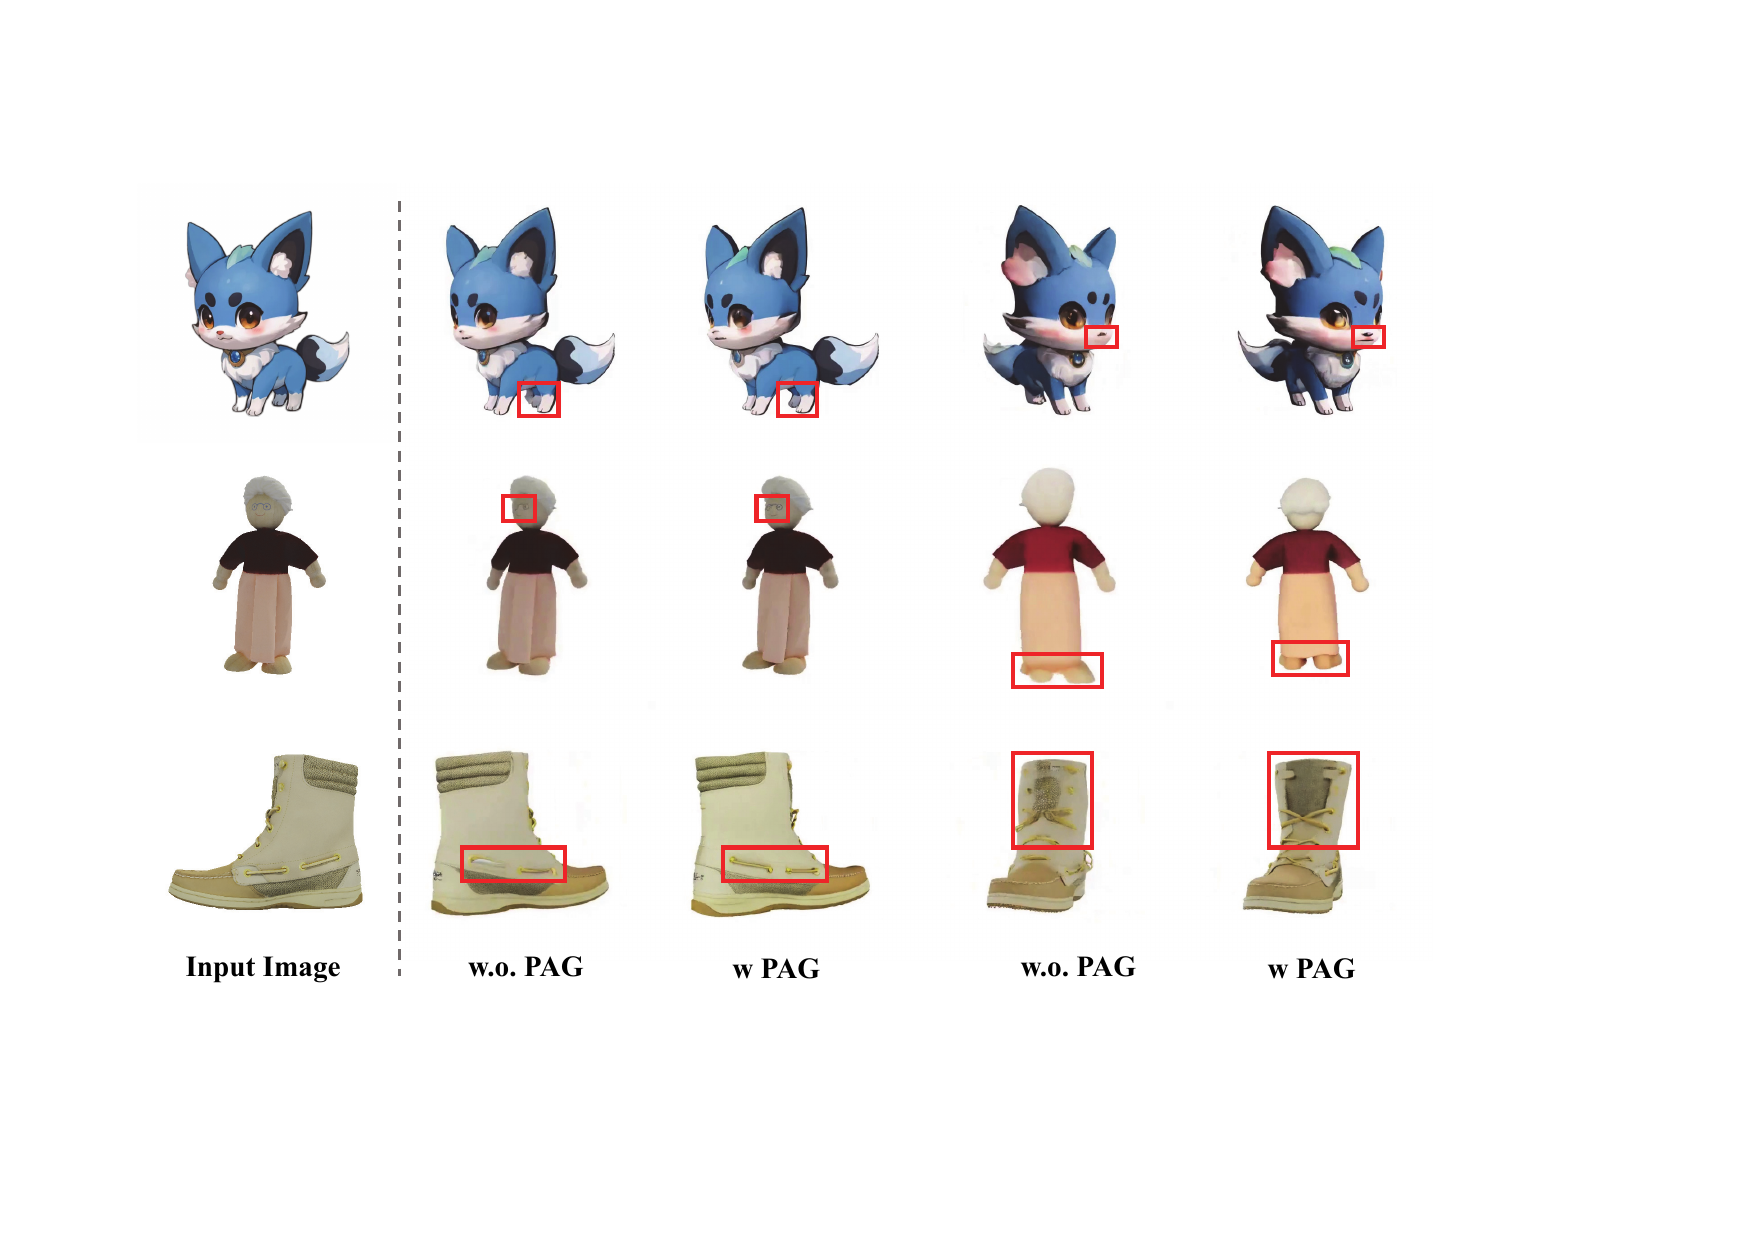}}
\caption{Impact of Perturbed-Attention Guidance (PAG). PAG enhances structural coherence and texture details, improving the visual quality across the generated multi-view frames.  {In this example, red bounding boxes highlight the quality improvements introduced by PAG in specific image regions.}
}
\label{fig:suppl_ablation_pag}
\end{figure*}

\begin{table*}[!t]
\caption{User Study. 
We curate a set of 30 samples and conduct a user study with 35 participants, each tasked with selecting the top two results that best matched the input image and exhibited the highest visual quality. Our method achieved the highest preference score, demonstrating its capability to produce visually compelling 3D assets.}
\label{table:user_study}
\small
\centering
\begin{tabular}{c|cccccc}
\toprule
Methods & TriplaneGaussian~\cite{triplanegaussian} & LGM~\cite{lgm} & DreamGaussian~\cite{dreamgaussian} & V3D~\cite{v3d} & Hi3D~\cite{hi3d} & Ours \\
\midrule
Preference$\uparrow$ & 19.81\% & 46.95\% & 25.14\% & 19.24\% & 21.91\% & \textbf{66.95\%} \\
\bottomrule
\end{tabular}
\end{table*}

\begin{figure*}[!t]
\centerline{\includegraphics[width=0.85\textwidth]{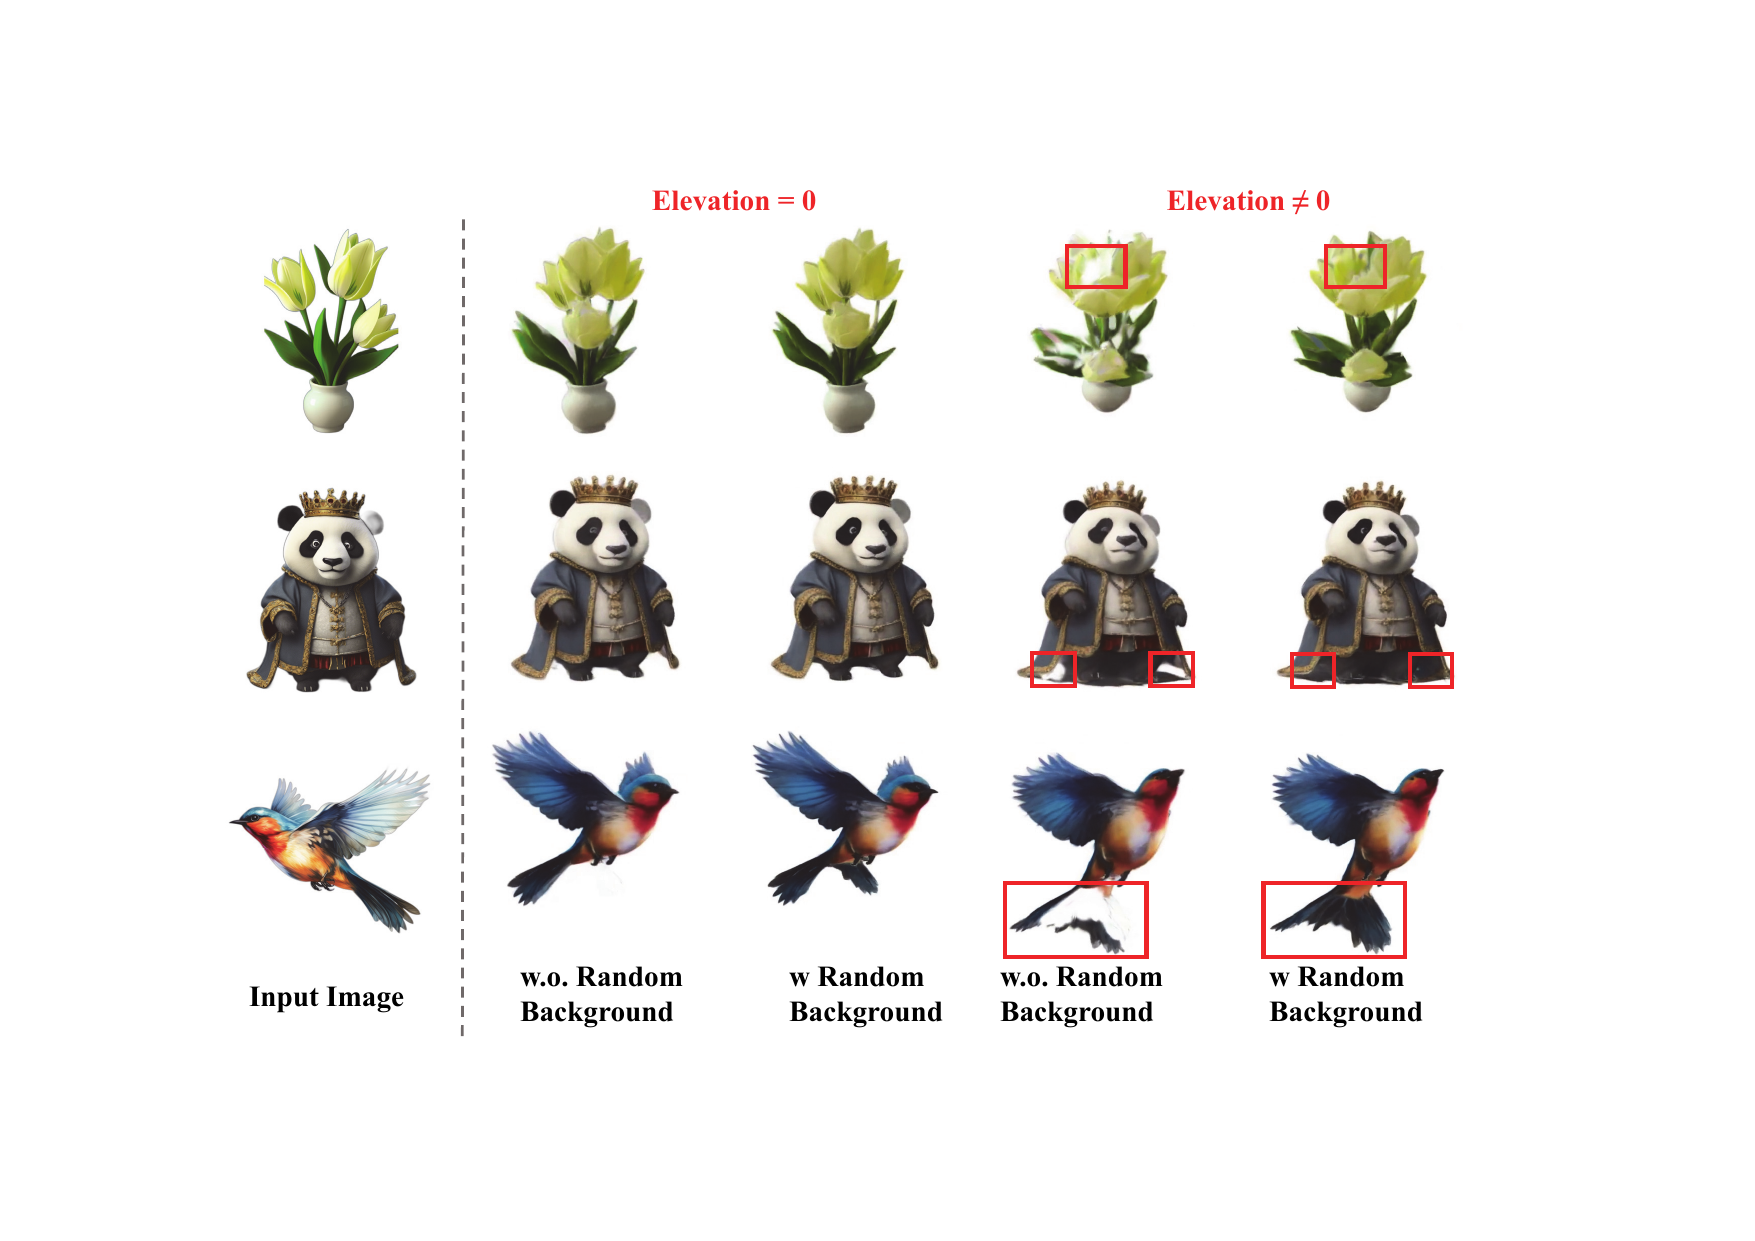}}
\caption{Impact of Random Background. 
{Red bounding boxes highlight the phenomenon of redundant white Gaussian points, which are barely noticeable at an elevation of 0 but become highly apparent at non-zero elevations.}
Randomly sampling background colors effectively reduces the densification of redundant white Gaussian points, improving the overall visual quality.
} 
\label{fig:suppl_ablation_random_bg}
\end{figure*}

\section{Visualization of Uncertainty}
As shown in Figure \ref{fig:suppl_vis_uncert}, we visualize the estimated uncertainty map, which follows min-max normalization for clarity. 
Intuitively, inconsistencies in the pseudo labels typically arise along object edges and sharp-textured regions, where inter-frame discrepancies induce conflicting supervision, leading to artifacts and floats. 
Our uncertainty map captures these inconsistencies effectively, highlighting higher uncertainty values in areas with sharp textures and edges.
By incorporating uncertainty regularization into the optimization process, we  mitigate the adverse effects of these inconsistencies on the generated 3D asset, significantly reducing artifacts and floats.

\section{Discussion of Uncertainty Regularization}
We dynamically adjust the pixel-wise loss weights using the uncertainty map. 
A natural question arises: why not incorporate the uncertainty map into the D-SSIM~\cite{ssim} and LPIPS~\cite{lpips} losses?
Both D-SSIM and LPIPS losses are employed to quantify the error between rendered images and pseudo-labels, aligning with the goal of the pixel-wise loss.
However, our experiments show that incorporating uncertainty information into these losses offers little improvement and, in some cases, even degrades performance.
We hypothesize that this happens because both D-SSIM and LPIPS focus on overall structural and perceptual consistency, rather than pixel-level details. 
As a result, they inherently handle inconsistencies between pseudo-labels at a higher level (such as texture and shape), without the need for fine-grained adjustments like incorporating uncertainty at the pixel level.
By instead incorporating the uncertainty map into pixel-wise regularization, we effectively mitigate the impact of pseudo-label inconsistencies.

\section{Additional Ablation Analysis}
\noindent\textbf{Impact of Perturbed-Attention Guidance (PAG). } 
In our approach, we employ SV3D~\cite{sv3d} to generate frames across a wide range of viewpoints. 
However, some generated samples exhibit distorted geometry or blurred textures.
To address these issues, we integrate PAG~\cite{pag} into SV3D, which enhances generation quality by guiding the denoising process away from the artificially degraded samples. 
As shown in Figure \ref{fig:suppl_ablation_pag}, the pseudo labels generated with PAG exhibit improved structure integrity and clearer, sharper textures.

\noindent\textbf{Impact of Random Background. } 
Figure \ref{fig:suppl_ablation_random_bg} demonstrates the effect of the random background strategy. 
In generated pseudo-labels, certain regions may be interpreted as foreground objects in some frames, while the same regions appear as background in others.
During the 3D asset optimization process, such inconsistencies may result in the densification of redundant white Gaussian points, which act as background elements.
These white Gaussian points are intended to occlude specific viewpoints to reconcile conflicting supervision, but they become conspicuously visible in additional rendered perspectives and may degrade visual quality.
To mitigate this, we adopted a random background strategy during training, where the background color is randomly selected rather than fixed as white. 
This approach effectively reduces the impact of  redundant white Gaussian points, significantly improving visual quality.

\section{User Study}
To evaluate visual quality, we curated a set of $30$ samples and conducted a user study with $35$ participants, as summarized in Table \ref{table:user_study}. 
Each participant was asked to select the top two results that best matched the input image and exhibited the highest visual quality, with the total preference score in the table summing to 200\%.
The collected preferences were then analyzed to compare the performance of our method with other state-of-the-art approaches.
As shown in the results, our method was selected more frequently than the other approaches, demonstrating its ability to consistently produce the most visually compelling 3D assets.
